# Supplementary material for: Measurement of reactor antineutrino oscillations with 1.46 ktonne-years of data at SNO+
Source: arXiv:2511.11856 ancillary file (2026-09-04)
Supplement: Supplementary file 1 [file Supplemental.pdf]

# SNO+ Experiment

## Supplemental Material

November 2025

This document provides supplemental information relevant to the measurement of reactor antineutrino oscillation in "Measurement of reactor antineutrino oscillation with 1.46 ktonne-years of data at SNO+".

## EVENT DISTRIBUTIONS

Figures 1-4 show parameter distributions of the selected IBD candidate events from the full dataset (top) and separate datasets I (bottom left) and II (bottom right). In Figs. 1-3, the data are compared with the predictions for signals and backgrounds, according to the best fit result in Fig. 7.

FIG. 1. Delayed event energy for the full dataset (top), and separate datasets I (bottom left) and II (bottom right).

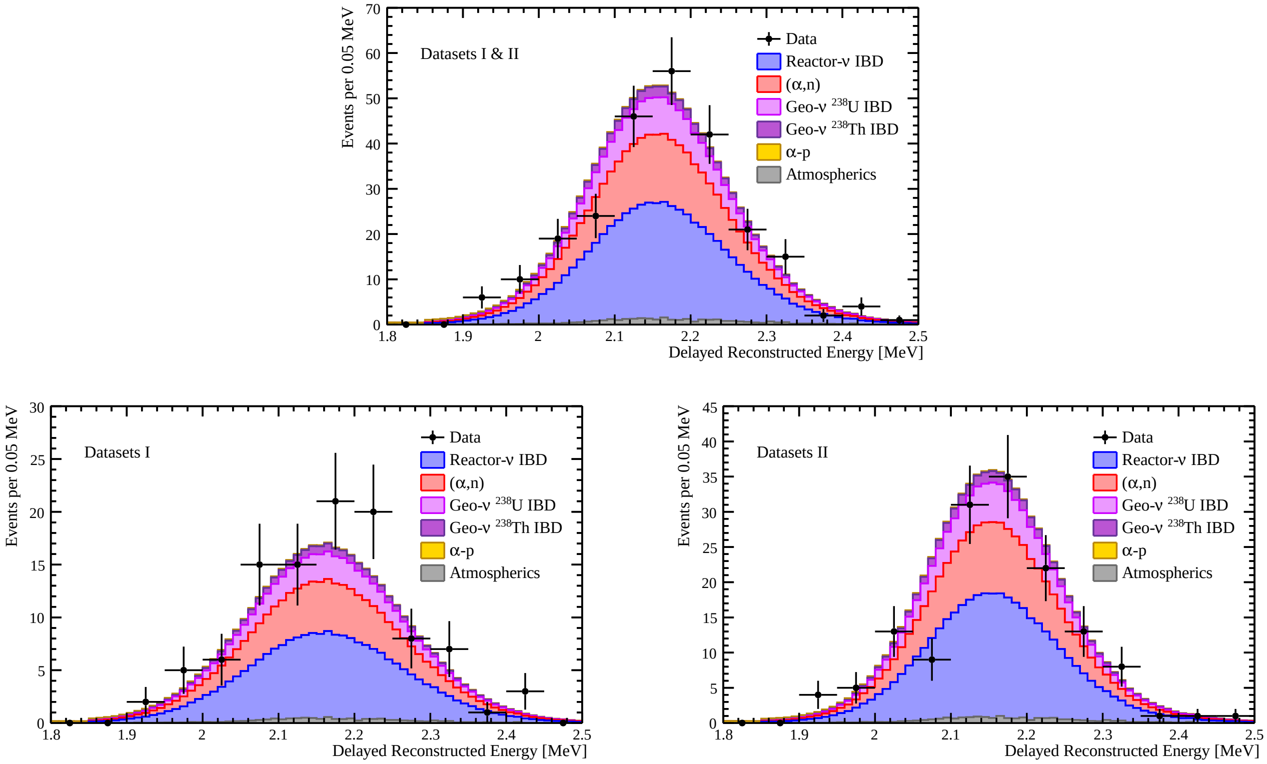

FIG. 2. Time between prompt and delayed events ($\Delta t$) for the full dataset (top), and separate datasets I (bottom left) and II (bottom right).

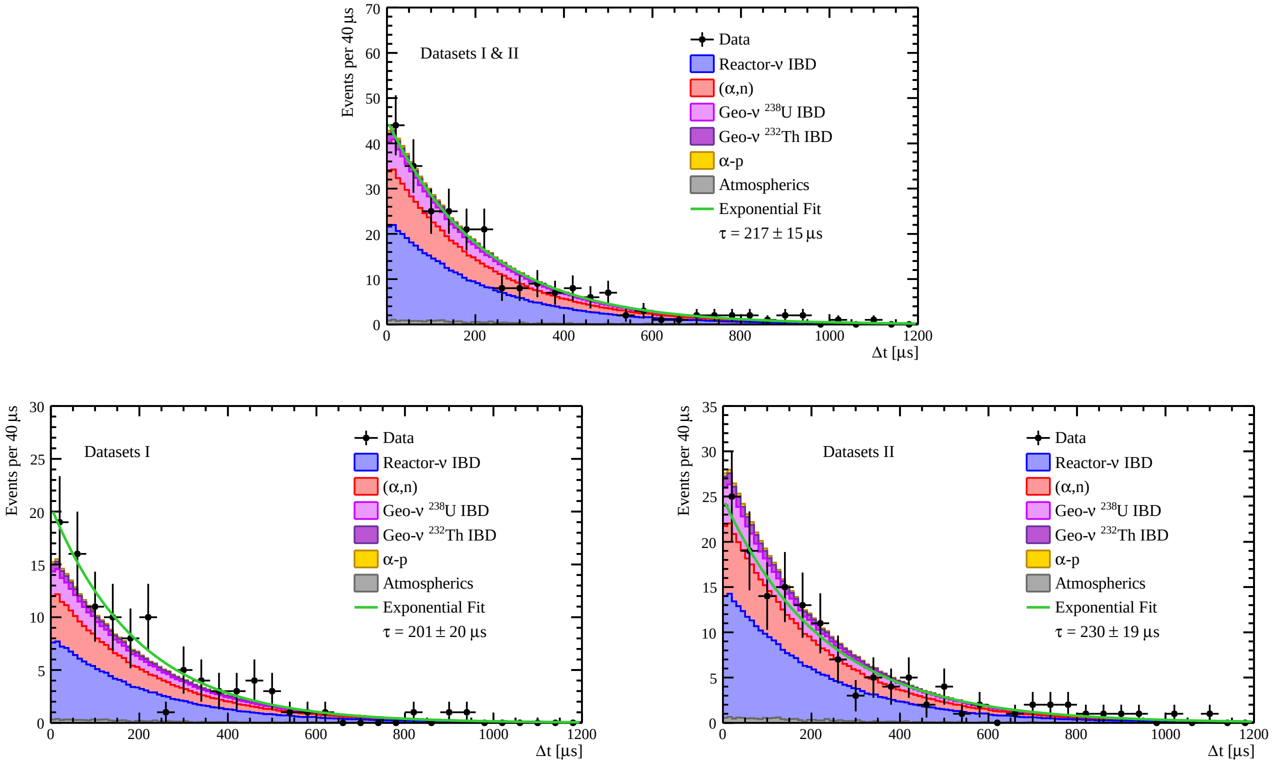


FIG. 3. Distance between prompt and delayed events ($\Delta r$) for the full dataset (top), and separate datasets I (bottom left) and II (bottom right).

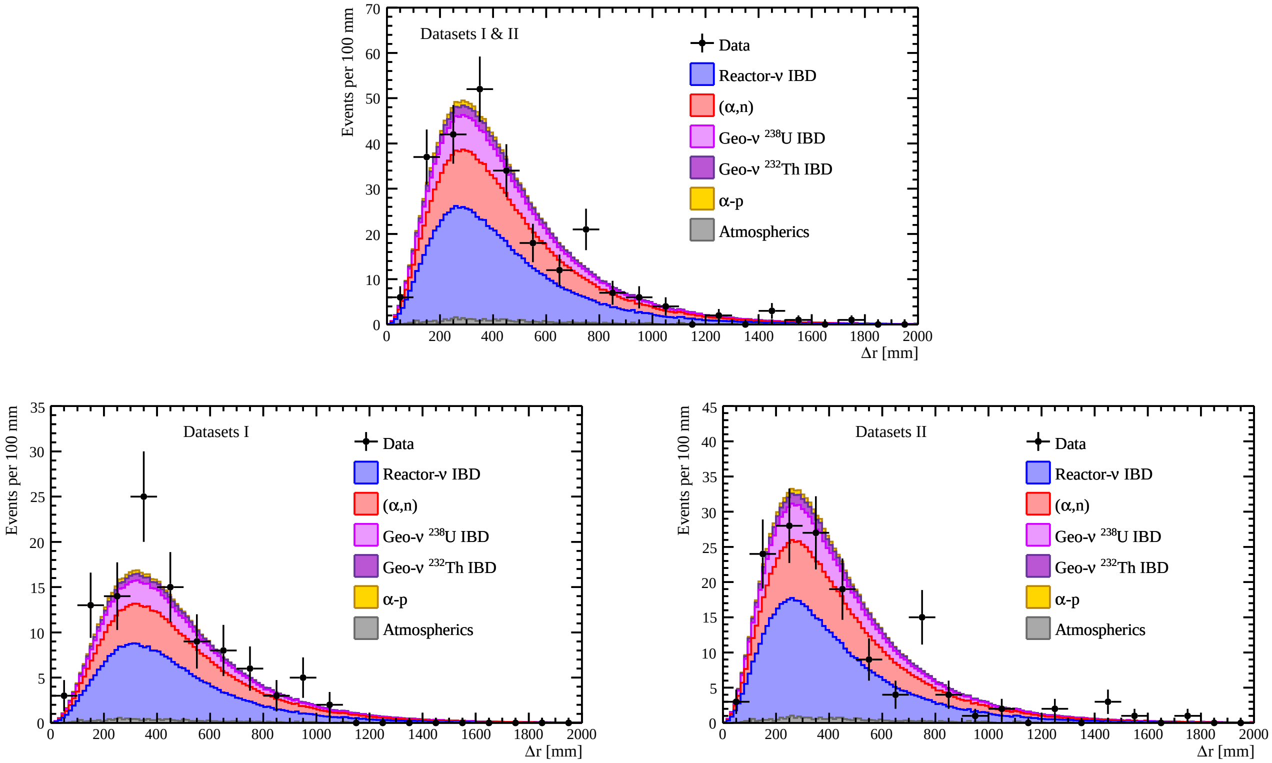

FIG. 4. Projections of the positions of selected coincident events for the full dataset (top), and separate datasets I (bottom left) and II (bottom right).

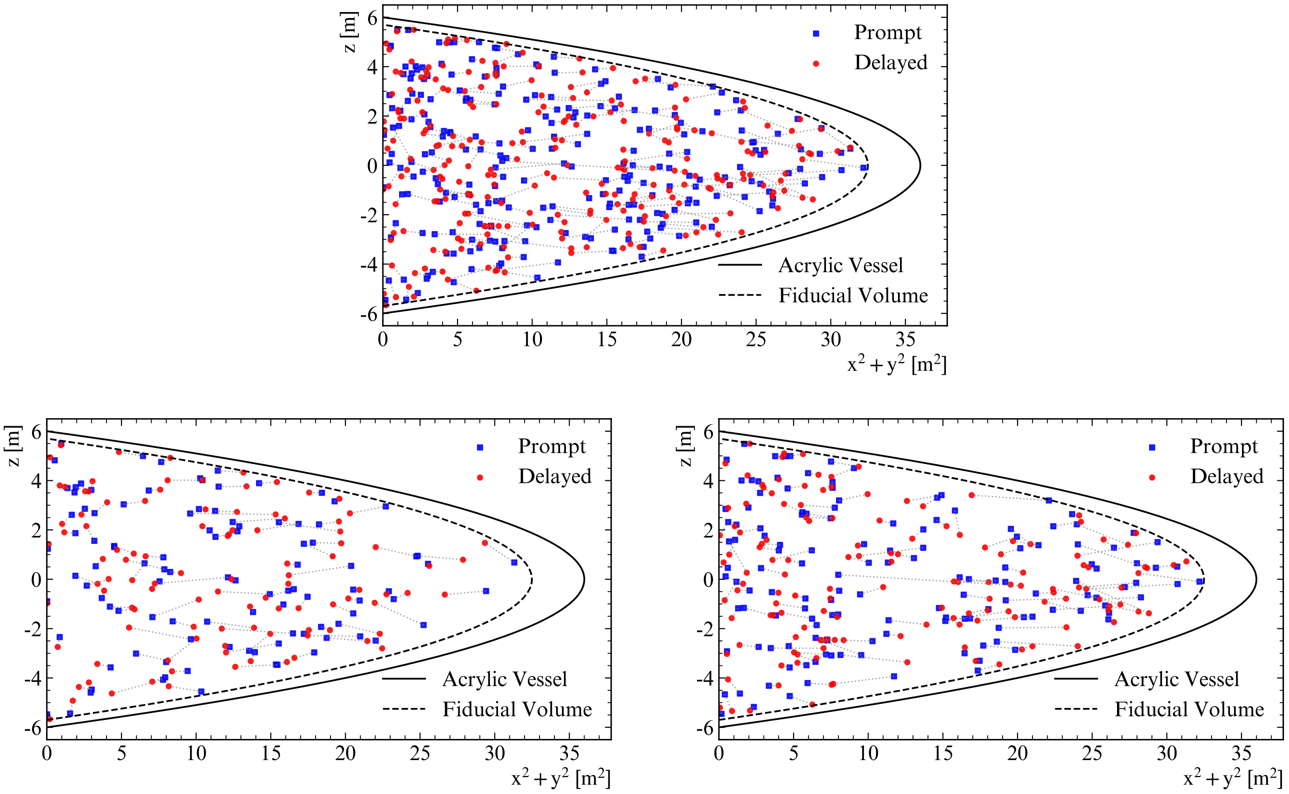


FIG. 5. Projections of the positions of selected coincident events for the full dataset.

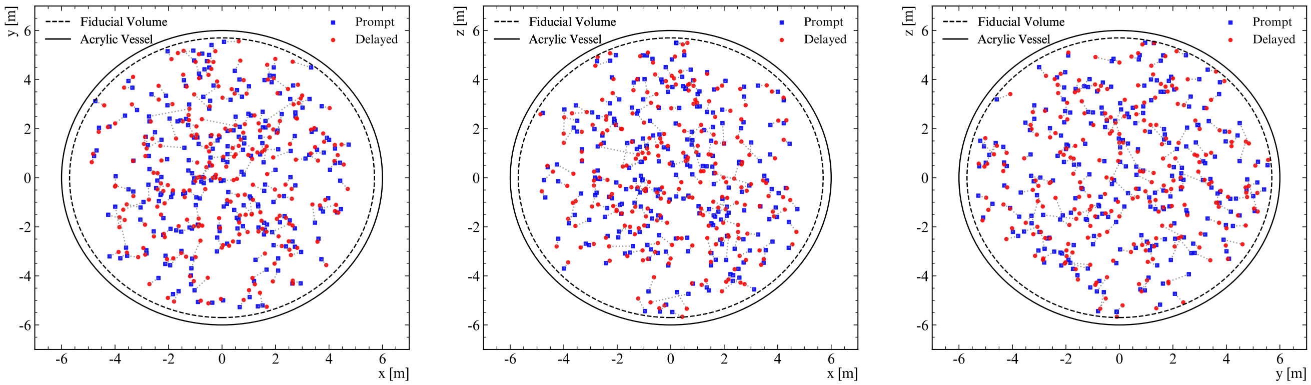

FIG. 6. $(\alpha, n)$ classification of $^{214}$Bi $\beta$'s and $^{214}$Po $\alpha$'s in the data and simulations (MC) of dataset II.

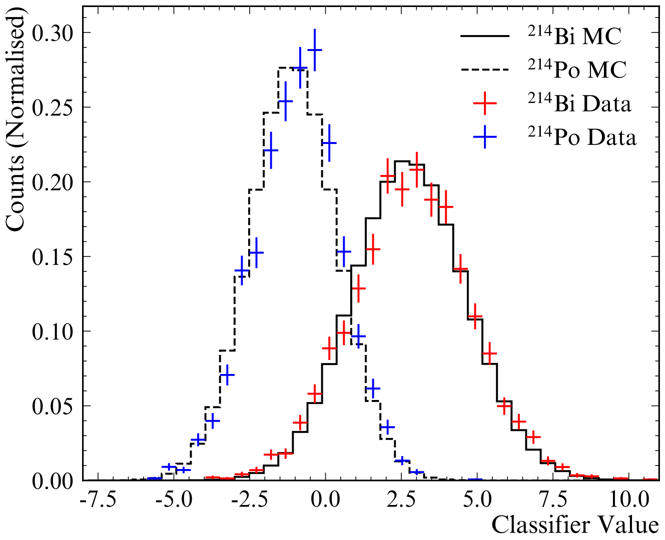

**FIT RESULTS**

FIG. 7. Full log-likelihood distribution from the unconstrained fit to the full SNO+ dataset.

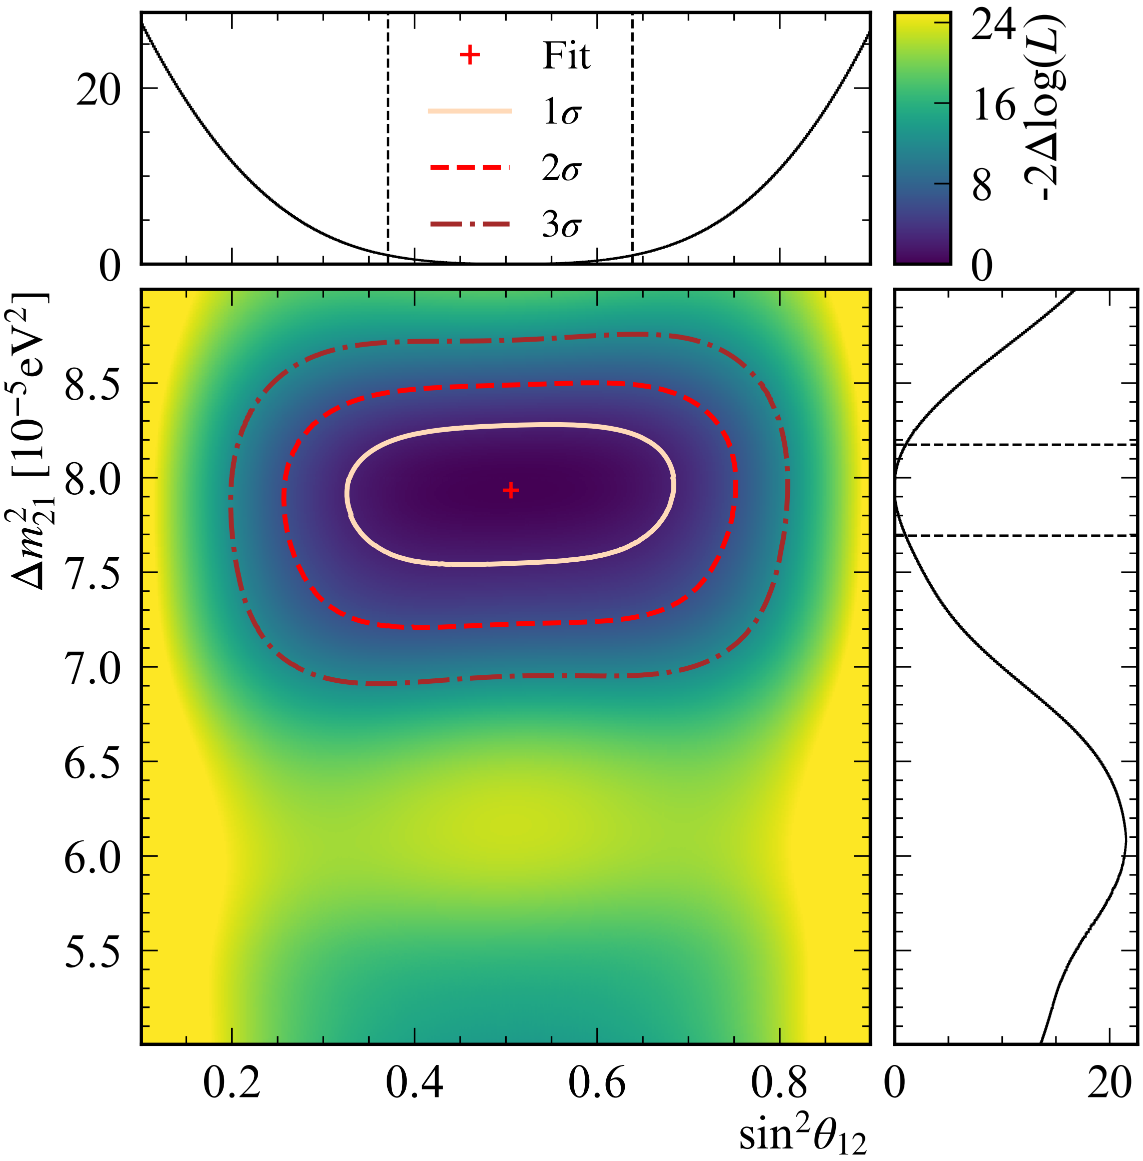

FIG. 8. Prompt energy spectra for the full dataset (top), and separate datasets I (bottom left) and II (bottom right), compared with expectations from the SNO+ unconstrained fit.

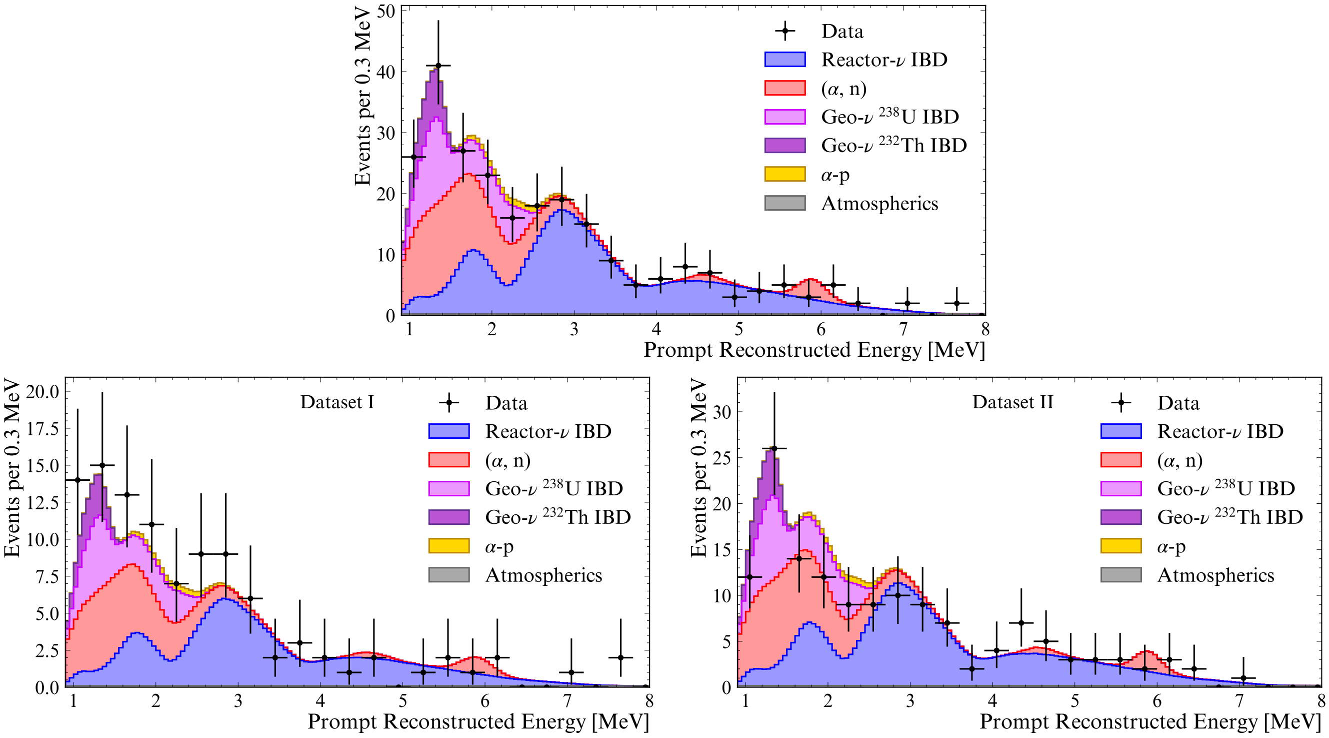


FIG. 9. Prompt energy spectra for the full dataset (top), and separate datasets I (bottom left) and II (bottom right), compared with expectations from the best fit to the SNO+ data with $\Delta m^2_{21}$ and $\sin^2\theta_{12}$ constrained using PDG 2025 values.

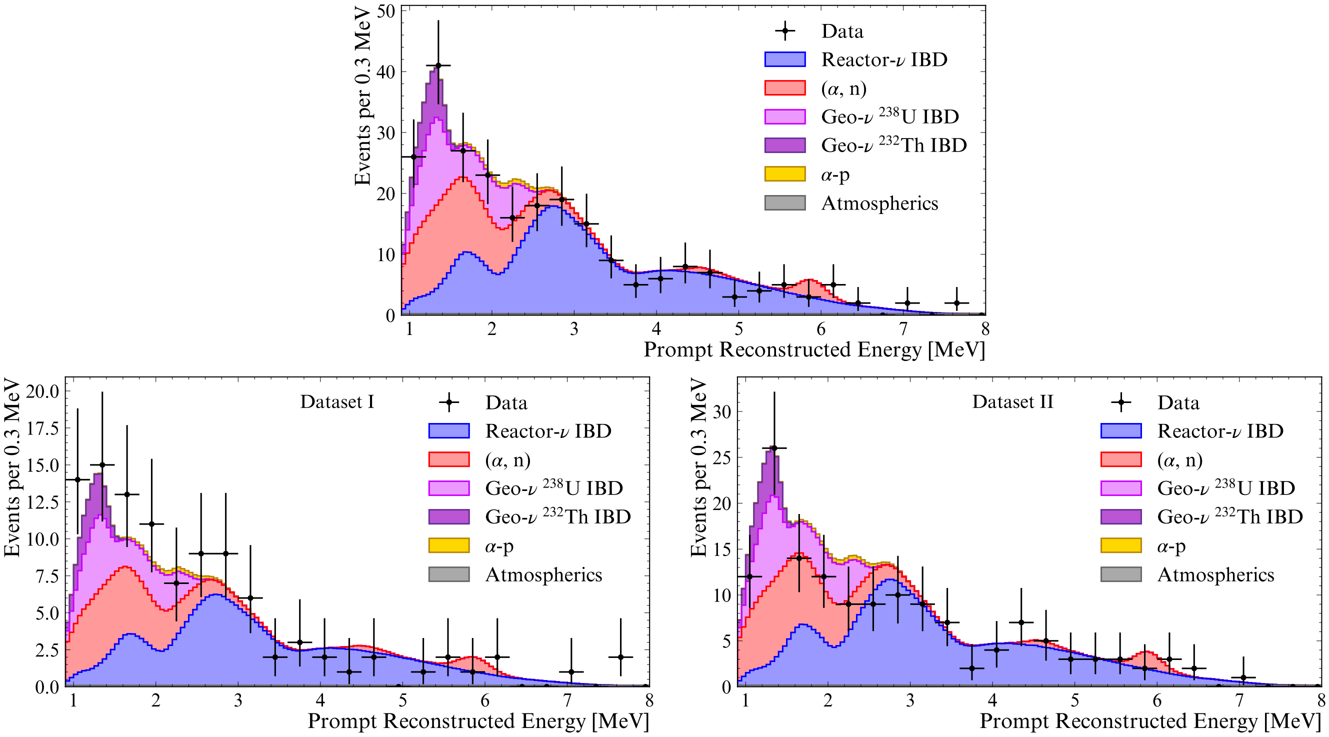

FIG. 10. Distributions of the $(\alpha, n)$ classifier value for prompt events with energy below 3.5 MeV, for the full dataset (top), and separate datasets I (bottom left) and II (bottom right). The classifier values are shifted to that the cut threshold for both datasets is at 0, denoted with a vertical dashed line in each case.

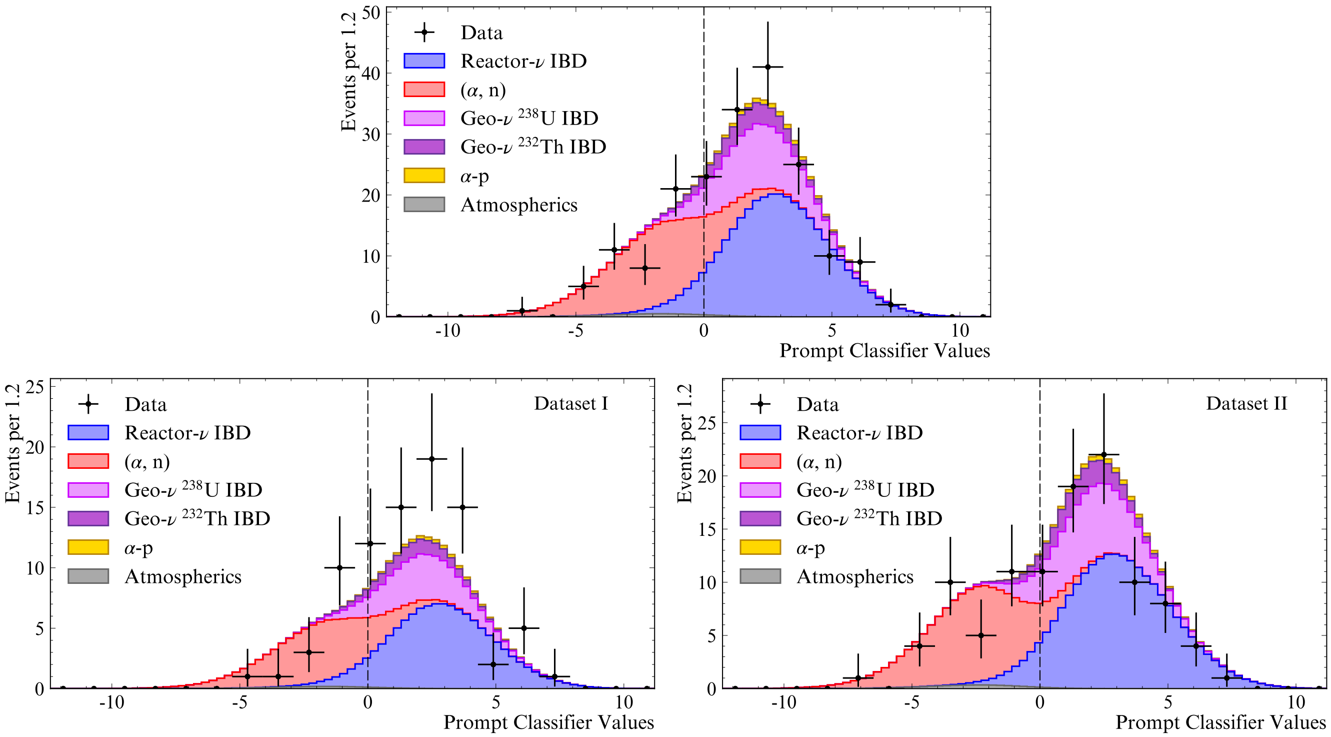


FIG. 11. Prompt energy spectra for the full dataset (top), and separate datasets I (bottom left) and II (bottom right), after applying the $(\alpha, n)$ classifier cut on prompt events with energy below 3.5 MeV. Data are compared with expectations from the best fit to the SNO+ data with the $(\alpha, n)$ cut applied and $\Delta m^2_{21}$ and $\sin^2\theta_{12}$ constrained using PDG 2025 values.

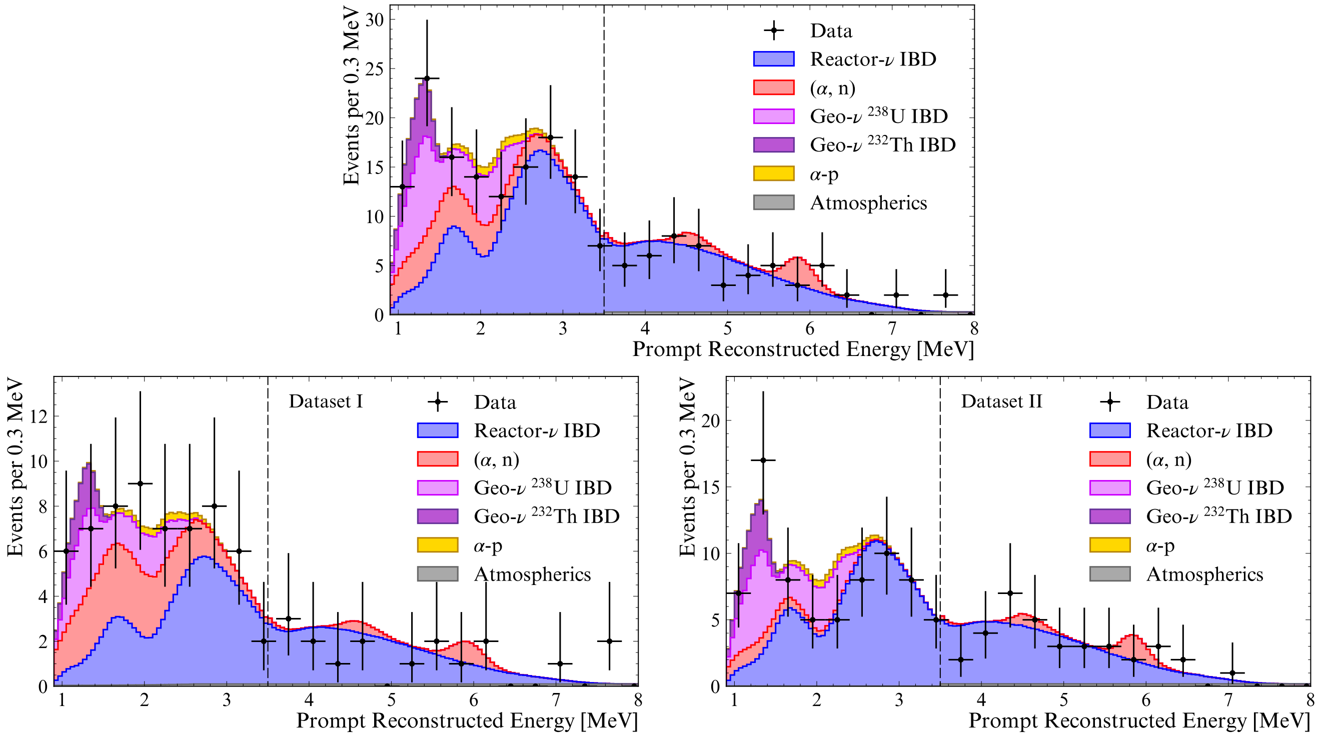

FIG. 12. Correlation matrices of the fit parameters, from the SNO+ fit (top left), fit with PDG 2025 constraints (top right), and the fit with PDG 2025 constraints and the $(\alpha, n)$ classifier cut on prompt events with energy below 3.5 MeV (bottom). The parameter symbols are defined in Table I, with "I" and "II" signifying the variables for datasets I and II, respectively.

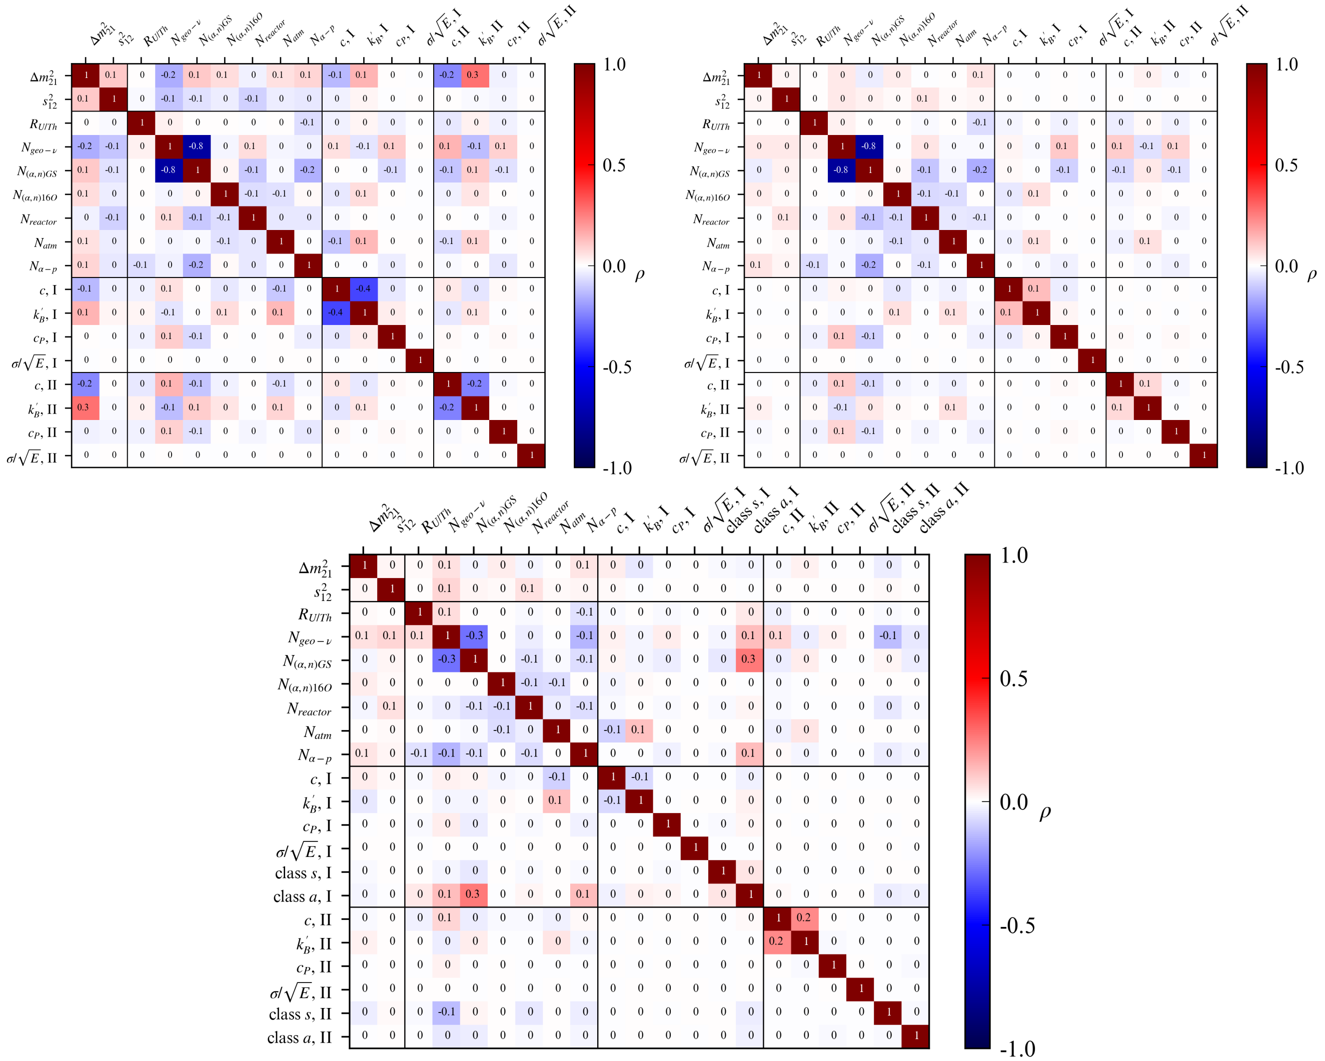

TABLE I. Summary of the floating parameters in the fits, in addition to the oscillation parameters $\Delta m^2_{21}$ and $s^2_{12} \equiv \sin^2\theta_{12}$. Constraints are applied as Gaussian penalty terms in the log-likelihood, except where otherwise stated. The normalizations act as scaling factors, scaling the associated PDFs of datasets I and II simultaneously. The other parameters only affect their respective dataset, as described in the first column. The linear energy scaling $c$ acts on all PDFs, while the extra scaling from $c_\mathrm{P}$ only acts on the $(\alpha, n)$ PDF below 3.5 MeV (proton scatters). In either case, the linear energy scaling acts on a PDF as $P'(E) = P(c\cdot E)$. The nonlinear energy scaling transforms PDFs via $P'(E) = P\left(\frac{1+k_B E}{1+k'_B E}E\right)$, where $k_B$ is fixed to 0.074 MeV$^{-1}$, and $k'_B$ is allowed to float about this value. The energy smearing is applied by convolving the PDFs with a Gaussian with $\sigma \propto \sqrt{E}$. Finally, the classifier parameters are only fit when the $(\alpha, n)$ classifier selection is used. The IBD classifier efficiency scaling $s$ is applied equally to the selection efficiency $\epsilon_i$ at every energy $E_i$ as $\epsilon'_i = s \cdot \epsilon_i$. The $(\alpha, n)$ classifier efficiency scaling is applied in an energy-dependent fashion, as $\epsilon'_i = \left(1 + a^2 \cdot E^3_i\right) \cdot \epsilon_i$.

| | Description | Symbol | Prior | Constraint |
|---|---|---|---|---|
| Normalizations | U/Th ratio | $R_{\mathrm{U/Th}}$ | 3.78 | 35% |
| | Geo-$\nu$ IBD | $N_{\text{geo-}\nu}$ | 1 | unconstrained, $\in [-100\%, +300\%]$ |
| | ($\alpha$, n) GS | $N_{(\alpha,\ \mathrm{n})\mathrm{GS}}$ | 1 | 30% |
| | ($\alpha$, n) ES | $N_{(\alpha,\ \mathrm{n})\mathrm{ES}}$ | 1 | 100% |
| | Reactor-$\nu$ IBD | $N_{\text{reactor-}\nu}$ | 1 | 4.3% |
| | Atmospheric $\nu$ | $N_{\mathrm{atm}}$ | 1 | 68% |
| | $\alpha$-p | $N_{\alpha-p}$ | 1 | 83% |
| Dataset I | Linear energy scaling | $c$ | 1 | 1.1% |
| | Nonlinear energy scaling | $k'_B$ | 0.074 MeV$^{-1}$ | 0.004 MeV$^{-1}$ |
| | Linear energy scaling for proton scatters | $c_\mathrm{P}$ | 1 | 3% |
| | Energy smearing | $\sigma/\sqrt{E}$ | 0 MeV$^{1/2}$ | 0.044 MeV$^{1/2}$ |
| | IBD classifier efficiency scaling | class $s$ | 1 | 2.9% |
| | $(\alpha, n)$ classifier efficiency scaling | class $a$ | 0 MeV$^{-3/2}$ | unconstrained, $\in [-0.67, 0.67]$ MeV$^{-3/2}$ |
| Dataset II | Linear energy scaling | $c$ | 1 | 1% |
| | Nonlinear energy scaling | $k'_B$ | 0.074 MeV$^{-1}$ | 0.004 MeV$^{-1}$ |
| | Linear energy scaling for proton scatters | $c_\mathrm{P}$ | 1 | 3% |
| | Energy smearing | $\sigma/\sqrt{E}$ | 0 MeV$^{1/2}$ | 0.049 MeV$^{1/2}$ |
| | IBD classifier efficiency scaling | class $s$ | 1 | 2.9% |
| | $(\alpha, n)$ classifier efficiency scaling | class $a$ | 0 MeV$^{-3/2}$ | unconstrained, $\in [-0.67, 0.67]$ MeV$^{-3/2}$ |
